# Supplementary material for: VERISCORE: Evaluating the factuality of verifiable claims in long-form text generation
Source: arXiv:2406.19276 source file (2024-06-27)
Supplement: Supplementary file 1 [file seemingly_plausible_claims.tex]

\section{Possibly hallucinated claim}\label{appendix:seemingly_plausible}

In \sectionref{subsec:issues}, we pointed that that there are model generated content that seems plausible. However, under scrutiny, they either need expertise to be judged or are likely to be hallucination. \tableref{tab:seemingly_plausible} gives one more example to illustrate such cases.

\begin{table*}[h]
\fontsize{10}{12}\selectfont
% \small
\centering 
\resizebox{\textwidth}{!}{%
\begin{tabular}{@{}p{16cm}@{}}
\toprule
\multicolumn{1}{c}{\textbf{\scalebox{1.1}{Example 1}}}
\\\midrule

\textbf{Claim}: Linguistic Citizenship views language use as a way of enacting disaffiliation with imagined communities.\newline

\textbf{Query 1}: What is linguistic citizenship\newline
\textbf{Result}: Linguistic Citizenship is an attempt to work through a blueprint for language for navigating living the complexities of a diverse and difficult world in conviviality (and convivial contest) with different Others.\newline

\textbf{Query 2}: What are imagined communities\newline
\textbf{Result}: Imagined communities refer to groups of people, not immediately tangible and accessible, with whom we connect through the power of the imagination. In our daily lives we interact with many communities whose existence can be felt concretely and directly … however, these are not the only communities with which we are affiliated … in imagining ourselves bonded with our fellow compatriots across space and time, we can feel a sense of community with people we have not met, but perhaps hope to meet one day.\newline

\textbf{Authors' note}: The search results using the claim itself as the query from Google Search do not mention \textit{linguistic citizenship} and \textit{imagined community} together. During the manual verification, beyond what Google Search already returned, we searched about \textit{linguistic citizenship} and \textit{imagined community}. The results are below. \newline
Based on the results, we sense that if one wants to disaffiliate with their imagined communities, they can simply stop imagining themselves bonded with such communities. ``Imagined community'' and ``use language as a way of enacting disaffiliation'' do not logically form a coherent connection.\newline \midrule

\multicolumn{1}{c}{\textbf{\scalebox{1.1}{Example 2}}}
\\\midrule

\textbf{Claim}: Japanese people encountered tigers in the form of stuffed animals before the Meiji era.\newline

\textbf{Original model response}: Before the Meiji era (1868-1912), Japanese people would encounter tigers mainly through artwork, literature, and other forms of media. They would also see tigers in zoos and circuses, as well as in the form of stuffed animals and other souvenirs.\newline

\textbf{Search result 1}\newline
Title: I've seen Japanese artwork from the Edo era and before depicting ...\newline
Content: ... Japanese person encounter a tiger before the Meiji era? ... Even baby tigers was captured and be made as stuffed. ... Are tigers semiaquatic animals ...\newline
Link: https://www.quora.com/I-ve-seen-Japanese-artwork-from-the-Edo-era-and-before-depicting-tigers-Did-tigers-ever-inhabit-the-islands-of-Japan-If-not-how-might-a-Japanese-person-encounter-a-tiger-before-the-Meiji-era\newline

\textbf{Search result 2}\newline
Title: I've seen Japanese artwork from the Edo era and before depicting ...\newline
Content: I've seen Japanese artwork from the Edo era and before depicting Tigers. Did tigers ever inhabit the islands of Japan?\newline
Link: https://www.reddit.com/r/AskHistorians/comments/p47bj6/ive\_seen\_japanese\_artwork\_from\_the\_edo\_era\_and/ \newline

\textbf{Authors' note}: We confirmed that the claim is faithfully extracted from the original model response (see below). The claim cannot be verified for two reasons. First, no search results (returned by different queries) directly mention ``stuffed tiger'' and ``Meiji era'' together. Only one search result mentions ``stuffed''. However, the \href{https://www.quora.com/Why-are-there-so-few-Siberian-tigers/answer/Dong-Yoon-Lee}{web page} does not mention the Meiji era. The second reason is that the claim is vague in the sense of what ``Japanese people'' means. The web page of search result 2 states that ``The Japanese came across tigers on their forays into Korea in the late 16th century.'' However, it is questionable whether the Japanese who conducted these forays represent ``Japanese people''. Given these reasons, we were not able to verify or falsify the claim.\newline
\bottomrule

\end{tabular}%
}
\caption{Examples of seemingly plausible but hard to be verified/falsified claims.}
\label{tab:seemingly_plausible}
\end{table*}
